# Supplementary material for: Parameterized complexity of computing maximum minimal blocking and hitting sets
Source: arXiv:2102.03404 source file (2021-02-05)
Supplement: Supplementary file 1 [file section_appendix_alphabeta.tex]

\subsection{Alternative \FPT algorithm for \MMHS/$(\alpha+\beta)$}.
\begin{definition}\label{def:mmhsfpt}
Let $\H$ be an hypergraph such that no hyperdge is included in another.
Given $H^* \in E(\H)$ and $v^* \in V(\H)$ we define $\H^{(v^*,H^*)}$ as follows.
Let $E'=\{H \in V(\H) \mid v^* \notin H\}$.
We define $V(\H^{(v^*,H^*)})=V(\H) \setminus H^*$ and $E(\H^{(v^*,H^*)})=\{H \setminus H^*, H \in E'\}$.
\end{definition}
Informally, $\H^{(v^*,H^*)}$ is obtained by removing vertices of $H^*$, removing any hyperedge containing $v^*$,  and modfying all the others are by removing from them vertices of $H^*$.
Hyperdges disjoint from $H^*$ are not modified, and hyperedges of size one (but not zero as no hyperedge is included in $H^*$) can appear.

\begin{lemma}\label{lemma:mmhsfpt}
Let $(\H,\beta)$ be an instance of \MMHS such that no hyperdge is included in another.
Let $H^* \in E(\H)$ and $v^* \in V(\H)$.
\begin{enumerate}
\item if $(\H^{(v^*,H^*)},\beta-1)$ is a yes-instance then $(\H,\beta)$ is a yes-instance \label{item1}
\item if $(\H,\beta)$ is a yes-instance and there exists a minimal hitting set $S$ such that \label{item2}
  \begin{itemize}
   \item $|S| \ge \beta$ and
   \item $S \cap H^* = \{v^*\}$,
   \end{itemize}
   then $(\H^{(v^*,H^*)},\beta-1)$ is a yes-instance 
\end{enumerate}
\end{lemma}

\begin{proof}
Let $E'=\{H \in V(\H) \mid v^* \notin H\}$. For any $H \in E'$, we know that $H \setminus H^* \in E(\H^{(v^*,H^*)})$, implying

Let us start with item~\ref{item1}.
Suppose that $(\H^{(v^*,H^*)},\beta-1)$ is a yes-instance, and let $S'$ be a minimal hitting set of $\H^{(v^*,H^*)}$ such that $|S'| \ge \beta-1$.
Let $S = S' \cup \{v^*\}$, and let us prove that $S$ is a minimal hitting set of $H$.
Let us first verify that $S$ is a hitting set of $H$.
that $S' \cap (H \setminus H^*) \neq \emptyset$, and thus that $S \cap H \neq \emptyset$. 
Moreover, for any $H \in E(\H) \setminus E'$, $v^* \in H$, implying also $S \cap H \neq \emptyset$.
Let us now verify that $S$ is minimal by finding for every $v \in S$ an hyperedge $H \in E(\H)$ such that $S \cap H = \{v\}$. 
For $v^*$, observe that $S' \cap H^* = \emptyset$, implying that $S \cap H^* = \{v^*\}$.
Let $v \in S$, $v \neq v^*$, implying that $v \in S'$. By minimality of $S'$ in $\H^{(v^*,H^*)}$, there exists $H' \in E(\H^{(v^*,H^*)})$ such that $S' \cap H' = \{v\}$.
By definition, $H' = H \setminus H^*$ for some $H \in E'$. As $S'\cap H^* = \emptyset$, we have $S' \cap H = S' \cap H' = \{v\}$.
As $v^* \notin H$, we get $S \cap H = S' \cap H = \{v\}$.

Let us now turn to item~\ref{item2} and suppose that there exists $S$ as stated.
Let $S' = S \setminus \{v^*\}$, and let us prove that $S'$ is a minimal hitting set of $\H^{(v^*,H^*)}$.
Let us first verify that $S'$ is a hitting set of $\H^{(v^*,H^*)}$.
Let $H' \in E(\H^{(v^*,H^*)})$. By definiton there exists $H \in E'$ such that $H' = H \setminus H^*$. As $S$ is a hitting set of $H$, there exists $v \in S \cap H$.
As $v^* \notin H$ we get that $v \neq v^*$. As $S \cap H^* = \{v^*\}$, we get that $v \notin H^*$, implying that $v \in H'$, and that $v \in S' \cap H'$.
Let us now verify that $S'$ is minimal by finding for every $v \in S'$ an hyperedge $H' \in E(\H^{(v^*,H^*)})$ such that $S' \cap H' = \{v\}$.
Let $v \in S'$. By minimality of $S$ in $\H$, there exists $H \in E(\H)$ such that $S \cap H = \{v\}$.
This implies that $v^* \notin H$, and thus that $H \in E'$  and $H' = H \setminus H^*$ is an hyperedge of $\H^{(v^*,H^*)}$. Thus, we get $S' \cap H' = \{v\}$ and we are done.
\end{proof}

\begin{theorem}\label{thm:algommhs}
We can decide an instance $(\H,\beta)$ of \MMHS in time \\$\O^*((\alpha(\H)\Delta(\H))^\beta)$,
where $\alpha(\H) = \max_{H \in E(\H)}|H|$ and $\Delta(\H) = \max_{v \in V(\H)}$ $|\{H \in E(\H) \mid v \in H\}|$.
\end{theorem}
\begin{proof}
Let us define a branching algorithm $A$ such that given an input $(\H,\beta)$ of \MMHS, $A(\H,\beta)$ returns true if and only if there exists a minimal
hitting set of $\H$ of size at least $\beta$.
If $\beta = 0$ then $\A$ returns true, and if $\beta > 0$ and $\H$ has no hyperedge, then $A$ returns false.

Let us now consider the non trivial case where $\beta > 0$ and $E(\H) \neq \emptyset$.
The algorithm starts by cleaning the hypergraph by removing in polynomial time any hyperedge $H \in E(\H)$ such that there exists $H' \in E(\H)$ with $H' \subseteq H$, leading to an equivalent instance
according to Property~\ref{prop:prelim} item~\ref{prop3}.
Now, let $H_0 \in E(\H)$.
Informally, $A$ guesses which vertex $v^* \in H$ is in a fixed optimal solution $S^*$, and which private hyperedge $H^*$ is such that $S^* \cap H^* = \{v^*\}$.
More formally, for any $v \in H_0$, let $E^{v} = \{H \in E(\H) \mid v \in H\}$.
Algorithm $A(\H,\beta)$ returns $\bigvee_{v \in H_0, H \in E^{v}}A(\H^{(v,H)},\beta-1)$.
Notice that the hypergraph $\H^{(v,H)}$ may have again hypeedges included in others, explaining why we cannot perform the cleaning step only once as a pre-processing step,
and why $A$ has to perform this cleaning step. \mb{it could be the case that when creating $\H^{(v,H)}$, an hyperedge $H$ will become $H'=H \setminus H^*$ by definition,
and then $H'$ will be removed as it contains another smaller hyperedge.. but I think there is no problem or special argument needed to treat this "chain reaction".}

Let us now prove the correctness of this case by induction on $\beta$.
Suppose $(\H,\beta)$ is a yes-instance, and let $S$ be a minimal hitting set of $\H$ where $|S| \ge \beta$.
As $S$ is a hitting set, there exists $v^* \in S \cap H_0$.
As $S$ is minimal, there exists $H^* \in E(\H)$ such that $S \cap H^* = \{v^*\}$.
According to Lemma~\ref{lemma:mmhsfpt}, this implies that $(\H^{(v,H)},\beta-1)$ is a yes-instance.
Moreover, as $H^* \in E^{v^*}$, there exists $v \in H_0, H \in E^{v}$ such that $(v,H)=(v^*,H^*)$, and thus by induction hypothesis $A(\H^{(v,H)},\beta-1)$ (and thus $A(\H,\beta)$) returns true.
The fact that if $A(\H,\beta)$ returns true implies that $(\H,\beta)$ is a yes-instance is immediate by induction hypothesis and using Lemma~\ref{lemma:mmhsfpt}.

The running time of the algorithm is straightforward as at any level on the recursion, we make a polynomial number of operations and we branch on $\{v \in H_0, H \in E^{v}\}$,
which has size at most $\alpha(\H)\Delta(\H)$.
\end{proof}
